# Supplementary material for: Moment Matching for Multi-Source Domain Adaptation
Source: arXiv:1812.01754 source file (2019-08-27)
Supplement: Supplementary file 1 [file 2_exp_on_sentiment_analysis.tex]

\clearpage
\subsection{Experiments on Sentiment Analysis}
\label{sec_sentiment}
In this section, we report experimental results on cross-domain sentiment analysis of text. We use Amazon review dataset~\cite{ref:blitzer}. The dataset contains four domains: Kitchen appliances, DVD, Books and Electronics. In each domain, there are 1000 positive and 1000 negative reviews from Amazon users. We follow the pre-processing procedure described in Gong et al~\cite{gong2013connecting}, which reduces the dimensionality of bag-of-words feature to use only 400 words, without losing performance. We leverage a fully connected neural network (with 400-128-32-2 units in each layer) as the sentiment classifier. \textit{Batch normalization}, \textit{relu} and \textit{dropout} techniques are applied. We apply our model to layer 3, \ie, the layer with 32 units. 

Multi-domain adaptation on sentiment analysis is under-explored, so we only compare our model to ``source combine'' baselines and \textit{Deep Adaptation Network}~\cite{long2015}. Table~\ref{tab_sentiment} shows the gain of our model from baselines. Our model \Name achieves a \textbf{82.4}\% average accuracy across four experiment settings and \NameB further boosts the result to \textbf{83.0}\%

\begin{table}[h]
	\center
	\begin{footnotesize}
		\begin{tabular}{p{1.1cm}|c|p{0.45cm}p{0.45cm}p{0.45cm}p{0.45cm}|p{0.45cm}}
			\multirow{2}{0cm}{Standards} &\multirow{2}{0cm}{Models} &\multirow{2}{0cm}{\begin{tiny}B,D,E\\$\rightarrow$K\end{tiny}} &\multirow{2}{0cm}{\begin{tiny}B,D,K\\$\rightarrow$E\end{tiny}} &\multirow{2}{0cm}{\begin{tiny}B,E,K\\$\rightarrow$D\end{tiny}} &\multirow{2}{0cm}{\begin{tiny}D,E,K\\$\rightarrow$B\end{tiny}} &\multirow{2}{0cm}{Avg} \\ &&&&&& \\
			\hline
			\multirow{2}{0.3cm}{Source combine}	&Source only&	77.9	&	79.2& 77.3	& 78.2	  &	 78.2	\\
			&DAN~\cite{long2015} 		&	81.2	&	82.9	& 79.3	& 80.5 	& 80.9	\\
			\hline													
			\multirow{5}{0.3cm}{Multi-Source}
			&Source only & 75.4  & 79.3 &74.5 &72.4 & 75.4\\				
			&DAN~\cite{long2015}	&	80.4	&	83.3	&	77.8 & \textbf{81.1}  	& 80.7	\\
			&DCTN~\cite{xu2018deep} & 81.5 & 82.2 & 80.8 & 79.5 & 81.0 \\
			&\Name(ours)	&\textbf{81.7}	&\textbf{86.2}		&\textbf{81.2}	&80.5		  &	\textbf{82.4}	\\
% 			\Xhline{1.0pt}
		\end{tabular}
	\end{footnotesize}
\caption{\textbf{Results on Sentiment Analysis}. B,D,E and K indicate \textit{Books}, \textit{DVD}, \textit{Electronics} and \textit{Kitchen appliances}, respectively. }
\label{tab_sentiment}
\end{table}

\noindent \textbf{Ablation Study}
The moment matching component in our model contains two parts: aligning multi-source domains with target domain and aligning source domains with each other. To demonstrate the importance of matching the source domains, we conduct two set of experiments on sentiment analysis, \ie \textit{w} or \textit{w/o} align the source domains. The results are shown in Table~\ref{tab_sentiment_ablation}. The performance will drop if the source domains are not aligned.

\begin{table}[h]
	\center
	\begin{footnotesize}
		\begin{tabular}{p{0.65cm}|p{1cm}p{1cm}p{1cm}p{1cm}|p{0.65cm}}
		  %  \Xhline{1.0pt}
		     & \begin{tiny}B,D,E$\rightarrow$K\end{tiny}
		     & \begin{tiny}B,D,K$\rightarrow$E\end{tiny}
		     & \begin{tiny}B,E,K$\rightarrow$D\end{tiny}
		     & \begin{tiny}D,E,K$\rightarrow$B\end{tiny}
		     & Avg\\
		     \hline
		     w & 81.7 & 86.2 & 81.2 & 80.5 & 82.4 \\
		     w/o & 80.1 & 85.8 & 79.8 & 78.5 & 80.3\\
% 			\Xhline{1.0pt}
		\end{tabular}
	\end{footnotesize}
\caption{Ablation study on sentiment analysis experiment. The performance will drop if the source domains are not aligned. \textit{w} and \textit{w/o} denote ``with aligning the source domains" or ``without".}
\label{tab_sentiment_ablation}
\end{table}
